# Supplementary material for: Self-supervised Multi-future Occupancy Forecasting for Autonomous Driving
Source: arXiv:2407.21126 source file (2025-10-17)
Supplement: Supplementary file 1 [file appendix.tex]

\section{Hyperparameteres}
\label{sec:implementation_details}
\subsection{Encoder \& Decoder}
\begin{table}[h]
    \centering
    \caption{Representation Learning Hyperparameters}
    \label{tab:hyperparams_rl}
    \begin{tabular}{@{}lr@{}} %{lX}
        \toprule
        \textbf{Parameter} & \textbf{Value} \\ 
        \midrule
        Architecture & ResNet \\
        Image Size & 1 $\times 128 \times 128$ \\
        Latent Dim L-OGM & $64 \times 4 \times 4$ \\
        Latent Dim Camera & $16 \times 4 \times 4$ \\
        Latent Dim Maps & $16 \times 4 \times 4$ \\
        Channel Multiplier & 2 \\
        Optimizer & Adam(lr=0.0001) \\
        Batch size & 24 per GPU \\
        KL reg $\beta$ & 50.0 \\
        Adv weight $\gamma$ & 1.0 \\
        Path reg & 2.0 \\
        Discriminator R1 reg & 10.0 \\
        GPUS & 4 NVIDIA V100 32 GB \\ 
        \bottomrule
    \end{tabular}
\end{table}
\subsection{Prediction Network}
\Cref{tab:hyperparams_stoch_pred} contains the hyperparameters for stochastic prediction. The prediction network training consists of three stages: deterministic training, low regularization training, and high regularization training. During deterministic training stage, $z_{stoch}$ is sampled from the target distribution. During regularized training, $z_{stoch}$ is sampeld from the inference network.   
\begin{table}[h]
    \centering
    \caption{Stochastic Prediction Hyperparameters}
    \label{tab:hyperparams_stoch_pred}
    \begin{tabular}{@{}lr@{}} %{lX}
        \toprule
        \textbf{Parameter} & \textbf{Value} \\ 
        \midrule
        Architecture & Transformer \\
        $d_{embed}$ & 256 \\
        $N_{enc}$ & 2 \\
        $N_{dec}$ &  1 \\
        $N_{heads}$ & 2 \\
        $d_{feedforward}$ & 128 \\
        Dropout & 0.01 \\ 
        Optimizer & AdamW(lr=0.0004) \\
        Deterministic Epochs & 10 \\
        Low Reg Epochs & 10 \\
        KL reg low $\gamma$ &  0.0001 \\
        KL reg $\gamma$ & 0.001 \\
        GPU & 1 NVIDIA RTX TITAN 24 GB \\
        \bottomrule
    \end{tabular}
\end{table}

\section{Image Similarity Metric}
\label{sec:is}
The Image Similarity metric determines the picture distance function $\psi$ between two matrices $m_1$ and $m_2$ as follows~\cite{birk2006merging}:
\begin{equation}
\begin{split}
    \psi(m_1,m_2) = \sum_{c \in \mathcal{C}} d(m_1,m_2,c) + d(m_2,m_1,c) 
\end{split}
\end{equation}
where
\begin{equation}
\begin{split}
    d(m_1,m_2,c) = \frac{\sum_{m_1[p]=c} \text{min} \{\text{md}(p_1,p_2)|m_2[p_2]=c\}}{\#_c(m_1)}.
\end{split}
\end{equation}

\noindent $\mathcal{C}$ is a set of discretized values assumed by $m_1$ or $m_2$ which are: occupied, occluded, and free. $m_1[p]$ denotes the value $c$ of map $m_1$ at position $p=(x,y)$. $\text{md}(p_1,p_2)=|x_1 - x_2| + |y_1 - y_2|$ is the Manhattan distance between points $p_1$ and $p_2$.  $\#_c(m_1)= \#\{p_1 \mid m_1[p_1]=c\}$ is the number of cells in $m_1$ with value $c$.

\section{Additional Qualitative Results}
\Cref{fig:vae_vaegan_comp} compares VAE-GAN (used in our experiments) and VAE. Samples from VAE-GAN appear more realistic and have sharper occupied cells. Besides the qualitative preferences, the choice of representation learning framework does not translate to significant quantitative differences. 
\begin{figure}[h]
    \centering
    \centerline{\includegraphics[width=12.0cm]{Figures/VAE_vs_VAEGAN.png}}
    \caption{Comparison between VAE-GAN and VAE on Nuscenes.}
    \label{fig:vae_vaegan_comp}
\end{figure}
